# Supplementary material for: Modelling Assessment Rubrics through Bayesian Networks: a Pragmatic Approach
Source: arXiv:2209.05467 source file (2024-08-02)
Supplement: Supplementary file 1 [file 07_appendix.tex]

\appendix
\section{Appendix}

\begin{center}
\begin{longtable}{c|ccccccccc}
\caption{Pupil skill posterior probabilities for Model 1 (leak). The answers provided by the \begin{math}j\end{math}-th pupil are denoted as \begin{math}\bm{y}^{(j)}\end{math}.\label{tab:bn_topology1}}
& \multicolumn{9}{c}{\textbf{\begin{math}P(X_i=1|\bm{y}^{(j)})\end{math}}}\\ 
\begin{math}j\end{math}&{\footnotesize \begin{math}i=1\end{math}}&{\footnotesize \begin{math}i=2\end{math}}&{\footnotesize \begin{math}i=3\end{math}}&{\footnotesize \begin{math}i=4\end{math}}&{\footnotesize \begin{math}i=5\end{math}}&{\footnotesize \begin{math}i=6\end{math}}&{\footnotesize \begin{math}i=7\end{math}}&{\footnotesize \begin{math}i=8\end{math}}&{\footnotesize \begin{math}i=9\end{math}}\\ \hline
\endfirsthead

\multicolumn{10}{c}{{\tablename\ \thetable{} -- continued from previous page}} \\
& \multicolumn{9}{c}{\textbf{\begin{math}P(X_i=1|\bm{y}^{(j)})\end{math}}}\\ 
\begin{math}j\end{math}&{\footnotesize \begin{math}i=1\end{math}}&{\footnotesize \begin{math}i=2\end{math}}&{\footnotesize \begin{math}i=3\end{math}}&{\footnotesize \begin{math}i=4\end{math}}&{\footnotesize \begin{math}i=5\end{math}}&{\footnotesize \begin{math}i=6\end{math}}&{\footnotesize \begin{math}i=7\end{math}}&{\footnotesize \begin{math}i=8\end{math}}&{\footnotesize \begin{math}i=9\end{math}}\\ \hline
\endhead

\hline \multicolumn{10}{r}{{Continued on next page}} \\ 
\endfoot

\hline \hline
\endlastfoot

1	&	0.54	&	0.70	&	0.92	&	0.64	&	0.71	&	0.17	&	0.71	&	0.21	&	0.00	\\
2	&	0.54	&	0.70	&	0.99	&	0.65	&	0.94	&	1.00	&	0.78	&	0.99	&	0.23	\\
3	&	0.54	&	0.70	&	0.99	&	0.68	&	0.96	&	1.00	&	0.85	&	1.00	&	1.00	\\
4	&	0.54	&	0.70	&	0.99	&	0.68	&	0.96	&	1.00	&	0.88	&	1.00	&	1.00	\\
5	&	0.54	&	0.70	&	0.99	&	0.66	&	0.95	&	1.00	&	0.84	&	0.99	&	0.86	\\
6	&	0.54	&	0.70	&	0.99	&	0.65	&	0.94	&	1.00	&	0.65	&	0.94	&	0.00	\\
7	&	0.54	&	0.70	&	0.99	&	0.68	&	0.96	&	1.00	&	0.91	&	1.00	&	1.00	\\
8	&	0.54	&	0.70	&	0.99	&	0.65	&	0.94	&	1.00	&	0.83	&	1.00	&	0.97	\\
9	&	0.54	&	0.70	&	0.97	&	0.68	&	0.96	&	0.97	&	0.88	&	0.91	&	0.02	\\
10	&	0.54	&	0.70	&	0.99	&	0.68	&	0.96	&	1.00	&	0.91	&	1.00	&	1.00	\\
11	&	0.54	&	0.70	&	0.11	&	0.68	&	0.83	&	0.00	&	0.95	&	0.89	&	0.00	\\
12	&	0.54	&	0.70	&	0.82	&	0.69	&	0.97	&	0.00	&	0.75	&	0.00	&	0.00	\\
13	&	0.54	&	0.70	&	0.97	&	0.65	&	0.94	&	0.04	&	0.78	&	0.15	&	0.00	\\
14	&	0.54	&	0.70	&	0.94	&	0.69	&	0.97	&	1.00	&	0.92	&	1.00	&	0.01	\\
15	&	0.54	&	0.70	&	0.99	&	0.66	&	0.95	&	1.00	&	0.84	&	1.00	&	1.00	\\
16	&	0.54	&	0.70	&	0.99	&	0.69	&	0.97	&	1.00	&	0.94	&	1.00	&	1.00	\\
17	&	0.54	&	0.70	&	0.99	&	0.68	&	0.96	&	1.00	&	0.91	&	1.00	&	1.00	\\
18	&	0.54	&	0.70	&	0.99	&	0.68	&	0.96	&	1.00	&	0.85	&	1.00	&	1.00	\\
19	&	0.54	&	0.70	&	0.99	&	0.69	&	0.97	&	1.00	&	0.96	&	1.00	&	1.00	\\
20	&	0.54	&	0.70	&	0.99	&	0.68	&	0.96	&	1.00	&	0.88	&	1.00	&	1.00	\\
21	&	0.54	&	0.70	&	0.99	&	0.69	&	0.97	&	1.00	&	0.89	&	1.00	&	1.00	\\
22	&	0.54	&	0.70	&	0.99	&	0.68	&	0.96	&	1.00	&	0.88	&	1.00	&	1.00	\\
23	&	0.54	&	0.70	&	0.99	&	0.68	&	0.96	&	1.00	&	0.85	&	0.99	&	0.99	\\
24	&	0.54	&	0.70	&	0.02	&	0.65	&	0.11	&	0.00	&	0.72	&	0.00	&	0.00	\\
25	&	0.54	&	0.70	&	0.39	&	0.68	&	0.83	&	0.00	&	0.80	&	0.00	&	0.00	\\
26	&	0.54	&	0.70	&	0.99	&	0.65	&	0.94	&	0.99	&	0.83	&	0.98	&	0.33	\\
27	&	0.54	&	0.70	&	0.99	&	0.62	&	0.91	&	0.89	&	0.76	&	0.99	&	0.00	\\
28	&	0.54	&	0.70	&	0.00	&	0.62	&	0.02	&	0.00	&	0.69	&	0.00	&	0.00	\\
29	&	0.54	&	0.70	&	0.99	&	0.68	&	0.96	&	1.00	&	0.94	&	1.00	&	1.00	\\
30	&	0.54	&	0.70	&	0.00	&	0.62	&	0.00	&	0.00	&	0.62	&	0.00	&	0.00	\\
31	&	0.01	&	0.00	&	0.00	&	0.00	&	0.00	&	0.00	&	0.00	&	0.00	&	0.00	\\
32	&	0.54	&	0.70	&	0.01	&	0.65	&	0.11	&	0.00	&	0.72	&	0.00	&	0.00	\\
33	&	0.00	&	0.00	&	0.00	&	0.00	&	0.00	&	0.00	&	0.00	&	0.00	&	0.00	\\
34	&	0.54	&	0.70	&	0.01	&	0.65	&	0.11	&	0.00	&	0.65	&	0.00	&	0.00	\\
35	&	0.54	&	0.70	&	0.01	&	0.65	&	0.11	&	0.00	&	0.72	&	0.00	&	0.00	\\
36	&	0.54	&	0.70	&	0.06	&	0.66	&	0.44	&	0.00	&	0.84	&	0.02	&	0.00	\\
37	&	0.54	&	0.70	&	0.01	&	0.65	&	0.11	&	0.00	&	0.72	&	0.00	&	0.00	\\
38	&	0.54	&	0.70	&	0.00	&	0.64	&	0.02	&	0.00	&	0.71	&	0.00	&	0.00	\\
39	&	0.54	&	0.70	&	0.90	&	0.68	&	0.83	&	1.00	&	0.91	&	1.00	&	0.99	\\
40	&	0.54	&	0.02	&	0.00	&	0.07	&	0.00	&	0.00	&	0.00	&	0.00	&	0.00	\\
41	&	0.54	&	0.69	&	0.02	&	0.66	&	0.38	&	0.00	&	0.73	&	0.00	&	0.00	\\
42	&	0.54	&	0.70	&	0.01	&	0.65	&	0.11	&	0.00	&	0.72	&	0.00	&	0.00	\\
43	&	0.54	&	0.70	&	0.03	&	0.66	&	0.44	&	0.00	&	0.73	&	0.00	&	0.00	\\
44	&	0.54	&	0.00	&	0.00	&	0.00	&	0.00	&	0.00	&	0.00	&	0.00	&	0.00	\\
45	&	0.54	&	0.07	&	0.00	&	0.26	&	0.00	&	0.00	&	0.00	&	0.00	&	0.00	\\
46	&	0.54	&	0.00	&	0.00	&	0.01	&	0.00	&	0.00	&	0.00	&	0.00	&	0.00	\\
47	&	0.54	&	0.70	&	0.00	&	0.62	&	0.00	&	0.00	&	0.62	&	0.00	&	0.00	\\
48	&	0.54	&	0.02	&	0.00	&	0.06	&	0.00	&	0.00	&	0.00	&	0.00	&	0.00	\\
49	&	0.19	&	0.00	&	0.00	&	0.00	&	0.00	&	0.00	&	0.00	&	0.00	&	0.00	\\
50	&	0.54	&	0.70	&	0.01	&	0.65	&	0.11	&	0.00	&	0.65	&	0.00	&	0.00	\\
51	&	0.54	&	0.70	&	0.94	&	0.69	&	0.84	&	0.24	&	0.54	&	0.03	&	0.00	\\
52	&	0.54	&	0.70	&	0.94	&	0.69	&	0.97	&	0.95	&	0.89	&	0.93	&	0.00	\\
53	&	0.54	&	0.70	&	0.47	&	0.68	&	0.83	&	0.00	&	0.85	&	0.01	&	0.00	\\
54	&	0.54	&	0.70	&	0.99	&	0.68	&	0.96	&	1.00	&	0.88	&	1.00	&	1.00	\\
55	&	0.54	&	0.70	&	0.63	&	0.68	&	0.83	&	0.00	&	0.74	&	0.00	&	0.00	\\
56	&	0.54	&	0.70	&	0.99	&	0.65	&	0.94	&	1.00	&	0.65	&	0.94	&	0.00	\\
57	&	0.54	&	0.70	&	0.56	&	0.65	&	0.38	&	0.05	&	0.72	&	0.01	&	0.00	\\
58	&	0.54	&	0.70	&	0.99	&	0.68	&	0.96	&	1.00	&	0.74	&	0.98	&	0.29	\\
59	&	0.54	&	0.70	&	0.77	&	0.68	&	0.83	&	0.74	&	0.85	&	0.79	&	0.00	\\
60	&	0.54	&	0.70	&	0.96	&	0.68	&	0.96	&	0.91	&	0.88	&	0.91	&	0.00	\\
61	&	0.54	&	0.70	&	0.86	&	0.68	&	0.83	&	0.95	&	0.80	&	0.58	&	0.00	\\
62	&	0.54	&	0.70	&	0.99	&	0.65	&	0.94	&	1.00	&	0.78	&	0.99	&	0.23	\\
63	&	0.54	&	0.69	&	0.81	&	0.68	&	0.79	&	0.76	&	0.88	&	0.45	&	0.00	\\
64	&	0.54	&	0.31	&	0.00	&	0.62	&	0.00	&	0.00	&	0.25	&	0.00	&	0.00	\\
65	&	0.54	&	0.70	&	0.32	&	0.68	&	0.83	&	0.00	&	0.91	&	0.04	&	0.00	\\
66	&	0.54	&	0.69	&	0.38	&	0.66	&	0.38	&	0.01	&	0.84	&	0.01	&	0.00	\\
67	&	0.54	&	0.08	&	0.00	&	0.07	&	0.00	&	0.00	&	0.00	&	0.00	&	0.00	\\
68	&	0.54	&	0.70	&	0.01	&	0.65	&	0.11	&	0.00	&	0.78	&	0.00	&	0.00	\\
69	&	0.01	&	0.00	&	0.00	&	0.00	&	0.00	&	0.00	&	0.00	&	0.00	&	0.00	\\
70	&	0.54	&	0.31	&	0.00	&	0.64	&	0.00	&	0.00	&	0.33	&	0.00	&	0.00	\\
71	&	0.54	&	0.31	&	0.00	&	0.66	&	0.02	&	0.00	&	0.07	&	0.00	&	0.00	\\
72	&	0.54	&	0.70	&	0.99	&	0.65	&	0.94	&	1.00	&	0.72	&	0.98	&	0.00	\\
73	&	0.54	&	0.70	&	0.70	&	0.68	&	0.83	&	0.18	&	0.91	&	0.84	&	0.00	\\
74	&	0.54	&	0.70	&	0.03	&	0.65	&	0.11	&	0.00	&	0.78	&	0.00	&	0.00	\\
75	&	0.54	&	0.31	&	0.00	&	0.64	&	0.00	&	0.00	&	0.07	&	0.00	&	0.00	\\
76	&	0.54	&	0.70	&	0.86	&	0.62	&	0.66	&	0.00	&	0.62	&	0.00	&	0.00	\\
77	&	0.54	&	0.70	&	0.40	&	0.68	&	0.45	&	0.00	&	0.29	&	0.00	&	0.00	\\
78	&	0.54	&	0.31	&	0.00	&	0.28	&	0.03	&	0.00	&	0.35	&	0.00	&	0.00	\\
79	&	0.01	&	0.00	&	0.00	&	0.00	&	0.00	&	0.00	&	0.00	&	0.00	&	0.00	\\
80	&	0.54	&	0.70	&	0.01	&	0.65	&	0.11	&	0.00	&	0.65	&	0.00	&	0.00	\\
81	&	0.54	&	0.70	&	0.01	&	0.65	&	0.11	&	0.00	&	0.65	&	0.00	&	0.00	\\
82	&	0.54	&	0.70	&	0.97	&	0.69	&	0.97	&	0.99	&	0.81	&	0.64	&	0.00	\\
83	&	0.54	&	0.70	&	0.99	&	0.65	&	0.94	&	1.00	&	0.78	&	0.99	&	0.23	\\
84	&	0.54	&	0.70	&	0.82	&	0.66	&	0.79	&	0.11	&	0.73	&	0.08	&	0.00	\\
85	&	0.54	&	0.70	&	0.94	&	0.64	&	0.71	&	0.74	&	0.71	&	0.56	&	0.00	\\
86	&	0.00	&	0.00	&	0.00	&	0.00	&	0.00	&	0.00	&	0.00	&	0.00	&	0.00	\\
87	&	0.54	&	0.70	&	0.48	&	0.66	&	0.11	&	0.00	&	0.43	&	0.01	&	0.00	\\
88	&	0.54	&	0.70	&	0.92	&	0.69	&	0.97	&	0.22	&	0.85	&	0.16	&	0.00	\\
89	&	0.54	&	0.70	&	0.01	&	0.65	&	0.02	&	0.00	&	0.27	&	0.00	&	0.00	\\
90	&	0.54	&	0.31	&	0.69	&	0.65	&	0.74	&	0.71	&	0.34	&	0.06	&	0.00	\\
91	&	0.54	&	0.70	&	0.55	&	0.69	&	0.84	&	0.00	&	0.31	&	0.00	&	0.00	\\
92	&	0.54	&	0.70	&	0.99	&	0.65	&	0.94	&	1.00	&	0.72	&	0.98	&	0.00	\\
93	&	0.54	&	0.70	&	0.47	&	0.68	&	0.45	&	0.00	&	0.44	&	0.00	&	0.00	\\
94	&	0.54	&	0.70	&	0.98	&	0.68	&	0.10	&	0.00	&	0.04	&	0.00	&	0.00	\\
95	&	0.54	&	0.70	&	0.99	&	0.62	&	0.91	&	0.89	&	0.76	&	0.99	&	0.00	\\
96	&	0.54	&	0.70	&	0.92	&	0.69	&	0.13	&	0.00	&	0.02	&	0.00	&	0.00	\\
97	&	0.54	&	0.70	&	0.98	&	0.64	&	0.67	&	0.01	&	0.40	&	0.10	&	0.00	\\
98	&	0.54	&	0.08	&	0.00	&	0.07	&	0.00	&	0.00	&	0.00	&	0.00	&	0.00	\\
99	&	0.54	&	0.70	&	0.77	&	0.68	&	0.83	&	0.74	&	0.85	&	0.79	&	0.00	\\
100	&	0.54	&	0.70	&	0.01	&	0.65	&	0.11	&	0.00	&	0.72	&	0.00	&	0.00	\\
101	&	0.54	&	0.70	&	0.03	&	0.66	&	0.44	&	0.00	&	0.66	&	0.00	&	0.00	\\
102	&	0.54	&	0.70	&	0.01	&	0.65	&	0.11	&	0.00	&	0.65	&	0.00	&	0.00	\\
103	&	0.54	&	0.70	&	0.70	&	0.69	&	0.13	&	0.00	&	0.08	&	0.00	&	0.00	\\
104	&	0.54	&	0.70	&	0.01	&	0.65	&	0.11	&	0.00	&	0.72	&	0.00	&	0.00	\\
105	&	0.54	&	0.29	&	0.10	&	0.29	&	0.15	&	0.00	&	0.52	&	0.00	&	0.00	\\
106	&	0.54	&	0.70	&	0.99	&	0.68	&	0.96	&	1.00	&	0.80	&	0.99	&	0.98	\\
107	&	0.54	&	0.31	&	0.00	&	0.25	&	0.00	&	0.00	&	0.06	&	0.00	&	0.00	\\
108	&	0.54	&	0.70	&	0.06	&	0.66	&	0.44	&	0.00	&	0.66	&	0.00	&	0.00	\\
109	&	0.54	&	0.70	&	0.01	&	0.65	&	0.11	&	0.00	&	0.65	&	0.00	&	0.00	\\   

\end{longtable}
\end{center}

\begin{center}
\begin{longtable}{c|ccccccccc}
\caption{Pupil skill posterior probabilities for Model 3 (leak). The answers provided by the \begin{math}j\end{math}-th pupil are denoted as \begin{math}\bm{y}^{(j)}\end{math}.\label{tab:bn_topology2}}
& \multicolumn{9}{c}{\textbf{\begin{math}P(X_i=1|\bm{y}^{(j)})\end{math}}}\\ 
\begin{math}j\end{math}&{\footnotesize \begin{math}i=1\end{math}}&{\footnotesize \begin{math}i=2\end{math}}&{\footnotesize \begin{math}i=3\end{math}}&{\footnotesize \begin{math}i=4\end{math}}&{\footnotesize \begin{math}i=5\end{math}}&{\footnotesize \begin{math}i=6\end{math}}&{\footnotesize \begin{math}i=7\end{math}}&{\footnotesize \begin{math}i=8\end{math}}&{\footnotesize \begin{math}i=9\end{math}}\\ \hline
\endfirsthead

\multicolumn{10}{c}%
{{\tablename\ \thetable{} -- continued from previous page}} \\
& \multicolumn{9}{c}{\textbf{\begin{math}P(X_i=1|\bm{y}^{(j)})\end{math}}}\\ 
\begin{math}j\end{math}&{\footnotesize \begin{math}i=1\end{math}}&{\footnotesize \begin{math}i=2\end{math}}&{\footnotesize \begin{math}i=3\end{math}}&{\footnotesize \begin{math}i=4\end{math}}&{\footnotesize \begin{math}i=5\end{math}}&{\footnotesize \begin{math}i=6\end{math}}&{\footnotesize \begin{math}i=7\end{math}}&{\footnotesize \begin{math}i=8\end{math}}&{\footnotesize \begin{math}i=9\end{math}}\\ \hline
\endhead

\hline \multicolumn{10}{r}{{Continued on next page}} \\ 
\endfoot

\hline \hline
\endlastfoot

1	&	0.55	&	0.76	&	0.98	&	0.66	&	0.89	&	0.99	&	0.74	&	0.79	&	0.05	\\
2	&	0.55	&	0.76	&	1.00	&	0.68	&	0.97	&	1.00	&	0.82	&	1.00	&	1.00	\\
3	&	0.55	&	0.76	&	1.00	&	0.72	&	0.98	&	1.00	&	0.89	&	1.00	&	1.00	\\
4	&	0.55	&	0.76	&	1.00	&	0.72	&	0.98	&	1.00	&	0.92	&	1.00	&	1.00	\\
5	&	0.55	&	0.76	&	0.99	&	0.70	&	0.98	&	1.00	&	0.88	&	1.00	&	1.00	\\
6	&	0.55	&	0.76	&	1.00	&	0.68	&	0.97	&	1.00	&	0.68	&	0.97	&	0.83	\\
7	&	0.55	&	0.76	&	1.00	&	0.72	&	0.98	&	1.00	&	0.95	&	1.00	&	1.00	\\
8	&	0.55	&	0.76	&	1.00	&	0.68	&	0.97	&	1.00	&	0.87	&	1.00	&	1.00	\\
9	&	0.55	&	0.76	&	0.98	&	0.72	&	0.98	&	1.00	&	0.92	&	1.00	&	1.00	\\
10	&	0.55	&	0.76	&	1.00	&	0.72	&	0.98	&	1.00	&	0.95	&	1.00	&	1.00	\\
11	&	0.55	&	0.76	&	0.46	&	0.72	&	0.96	&	0.22	&	0.97	&	1.00	&	0.02	\\
12	&	0.55	&	0.76	&	0.86	&	0.74	&	0.99	&	0.14	&	0.81	&	0.13	&	0.00	\\
13	&	0.55	&	0.76	&	0.98	&	0.68	&	0.97	&	0.90	&	0.82	&	0.73	&	0.01	\\
14	&	0.55	&	0.76	&	0.96	&	0.74	&	0.99	&	1.00	&	0.95	&	1.00	&	1.00	\\
15	&	0.55	&	0.76	&	1.00	&	0.70	&	0.98	&	1.00	&	0.88	&	1.00	&	1.00	\\
16	&	0.55	&	0.76	&	1.00	&	0.74	&	0.99	&	1.00	&	0.96	&	1.00	&	1.00	\\
17	&	0.55	&	0.76	&	1.00	&	0.72	&	0.98	&	1.00	&	0.94	&	1.00	&	1.00	\\
18	&	0.55	&	0.76	&	1.00	&	0.72	&	0.98	&	1.00	&	0.89	&	1.00	&	1.00	\\
19	&	0.55	&	0.76	&	1.00	&	0.74	&	0.99	&	1.00	&	0.98	&	1.00	&	1.00	\\
20	&	0.55	&	0.76	&	1.00	&	0.72	&	0.98	&	1.00	&	0.92	&	1.00	&	1.00	\\
21	&	0.55	&	0.76	&	1.00	&	0.74	&	0.99	&	1.00	&	0.93	&	1.00	&	1.00	\\
22	&	0.55	&	0.76	&	1.00	&	0.72	&	0.98	&	1.00	&	0.92	&	1.00	&	1.00	\\
23	&	0.55	&	0.76	&	0.99	&	0.72	&	0.98	&	1.00	&	0.89	&	1.00	&	1.00	\\
24	&	0.55	&	0.76	&	0.36	&	0.68	&	0.69	&	0.07	&	0.75	&	0.04	&	0.00	\\
25	&	0.55	&	0.76	&	0.63	&	0.72	&	0.96	&	0.00	&	0.85	&	0.07	&	0.00	\\
26	&	0.55	&	0.76	&	0.99	&	0.68	&	0.97	&	1.00	&	0.87	&	1.00	&	1.00	\\
27	&	0.55	&	0.76	&	1.00	&	0.64	&	0.94	&	1.00	&	0.78	&	0.99	&	1.00	\\
28	&	0.55	&	0.76	&	0.09	&	0.64	&	0.27	&	0.00	&	0.72	&	0.00	&	0.00	\\
29	&	0.55	&	0.76	&	1.00	&	0.72	&	0.98	&	1.00	&	0.96	&	1.00	&	1.00	\\
30	&	0.55	&	0.76	&	0.03	&	0.64	&	0.16	&	0.00	&	0.64	&	0.00	&	0.00	\\
31	&	0.04	&	0.00	&	0.00	&	0.00	&	0.00	&	0.00	&	0.00	&	0.00	&	0.00	\\
32	&	0.55	&	0.76	&	0.12	&	0.68	&	0.69	&	0.00	&	0.76	&	0.00	&	0.00	\\
33	&	0.00	&	0.00	&	0.00	&	0.00	&	0.00	&	0.00	&	0.00	&	0.00	&	0.00	\\
34	&	0.55	&	0.76	&	0.12	&	0.68	&	0.69	&	0.00	&	0.68	&	0.00	&	0.00	\\
35	&	0.55	&	0.76	&	0.12	&	0.68	&	0.69	&	0.00	&	0.76	&	0.00	&	0.00	\\
36	&	0.55	&	0.76	&	0.44	&	0.70	&	0.87	&	0.45	&	0.88	&	0.84	&	0.00	\\
37	&	0.55	&	0.76	&	0.12	&	0.68	&	0.69	&	0.00	&	0.76	&	0.00	&	0.00	\\
38	&	0.55	&	0.76	&	0.04	&	0.66	&	0.34	&	0.00	&	0.74	&	0.00	&	0.00	\\
39	&	0.55	&	0.76	&	0.98	&	0.72	&	0.96	&	1.00	&	0.95	&	1.00	&	1.00	\\
40	&	0.55	&	0.07	&	0.00	&	0.16	&	0.00	&	0.00	&	0.00	&	0.00	&	0.00	\\
41	&	0.55	&	0.74	&	0.20	&	0.70	&	0.83	&	0.00	&	0.78	&	0.00	&	0.00	\\
42	&	0.55	&	0.76	&	0.16	&	0.68	&	0.69	&	0.00	&	0.76	&	0.00	&	0.00	\\
43	&	0.55	&	0.76	&	0.26	&	0.70	&	0.89	&	0.00	&	0.77	&	0.00	&	0.00	\\
44	&	0.55	&	0.00	&	0.00	&	0.00	&	0.00	&	0.00	&	0.00	&	0.00	&	0.00	\\
45	&	0.55	&	0.11	&	0.00	&	0.24	&	0.00	&	0.00	&	0.01	&	0.00	&	0.00	\\
46	&	0.55	&	0.04	&	0.00	&	0.10	&	0.00	&	0.00	&	0.00	&	0.00	&	0.00	\\
47	&	0.55	&	0.76	&	0.02	&	0.64	&	0.16	&	0.00	&	0.64	&	0.00	&	0.00	\\
48	&	0.55	&	0.11	&	0.00	&	0.21	&	0.00	&	0.00	&	0.04	&	0.00	&	0.00	\\
49	&	0.26	&	0.00	&	0.00	&	0.00	&	0.00	&	0.00	&	0.00	&	0.00	&	0.00	\\
50	&	0.55	&	0.76	&	0.10	&	0.68	&	0.66	&	0.00	&	0.68	&	0.00	&	0.00	\\
51	&	0.55	&	0.76	&	0.97	&	0.74	&	0.96	&	0.99	&	0.78	&	0.84	&	0.02	\\
52	&	0.55	&	0.76	&	0.96	&	0.74	&	0.99	&	1.00	&	0.93	&	1.00	&	0.99	\\
53	&	0.55	&	0.76	&	0.75	&	0.72	&	0.96	&	0.12	&	0.89	&	0.69	&	0.00	\\
54	&	0.55	&	0.76	&	1.00	&	0.72	&	0.98	&	1.00	&	0.92	&	1.00	&	1.00	\\
55	&	0.55	&	0.76	&	0.83	&	0.72	&	0.96	&	0.56	&	0.79	&	0.26	&	0.00	\\
56	&	0.55	&	0.76	&	1.00	&	0.68	&	0.97	&	1.00	&	0.68	&	0.97	&	0.83	\\
57	&	0.55	&	0.76	&	0.90	&	0.68	&	0.82	&	0.99	&	0.76	&	0.55	&	0.00	\\
58	&	0.55	&	0.76	&	1.00	&	0.72	&	0.98	&	1.00	&	0.79	&	0.99	&	1.00	\\
59	&	0.55	&	0.76	&	0.93	&	0.72	&	0.96	&	1.00	&	0.89	&	0.99	&	0.23	\\
60	&	0.55	&	0.76	&	0.98	&	0.72	&	0.98	&	1.00	&	0.92	&	0.99	&	0.92	\\
61	&	0.55	&	0.76	&	0.97	&	0.72	&	0.96	&	1.00	&	0.85	&	0.97	&	0.86	\\
62	&	0.55	&	0.76	&	1.00	&	0.68	&	0.97	&	1.00	&	0.82	&	1.00	&	1.00	\\
63	&	0.55	&	0.74	&	0.95	&	0.72	&	0.95	&	1.00	&	0.92	&	0.97	&	0.84	\\
64	&	0.55	&	0.50	&	0.01	&	0.64	&	0.06	&	0.00	&	0.41	&	0.00	&	0.00	\\
65	&	0.55	&	0.76	&	0.61	&	0.72	&	0.96	&	0.01	&	0.94	&	0.91	&	0.00	\\
66	&	0.55	&	0.74	&	0.82	&	0.70	&	0.85	&	0.96	&	0.87	&	0.73	&	0.02	\\
67	&	0.55	&	0.15	&	0.01	&	0.13	&	0.00	&	0.00	&	0.00	&	0.00	&	0.00	\\
68	&	0.55	&	0.76	&	0.21	&	0.68	&	0.69	&	0.01	&	0.82	&	0.07	&	0.00	\\
69	&	0.04	&	0.00	&	0.00	&	0.00	&	0.00	&	0.00	&	0.00	&	0.00	&	0.00	\\
70	&	0.55	&	0.50	&	0.09	&	0.66	&	0.17	&	0.05	&	0.53	&	0.01	&	0.00	\\
71	&	0.55	&	0.50	&	0.08	&	0.70	&	0.26	&	0.00	&	0.16	&	0.00	&	0.00	\\
72	&	0.55	&	0.76	&	1.00	&	0.68	&	0.97	&	1.00	&	0.76	&	0.99	&	0.99	\\
73	&	0.55	&	0.76	&	0.90	&	0.72	&	0.96	&	0.99	&	0.94	&	1.00	&	0.96	\\
74	&	0.55	&	0.76	&	0.32	&	0.68	&	0.69	&	0.00	&	0.81	&	0.01	&	0.00	\\
75	&	0.55	&	0.50	&	0.01	&	0.66	&	0.04	&	0.00	&	0.19	&	0.00	&	0.00	\\
76	&	0.55	&	0.76	&	0.96	&	0.64	&	0.85	&	0.22	&	0.64	&	0.10	&	0.00	\\
77	&	0.55	&	0.76	&	0.80	&	0.72	&	0.88	&	0.66	&	0.51	&	0.04	&	0.00	\\
78	&	0.55	&	0.55	&	0.12	&	0.51	&	0.59	&	0.00	&	0.61	&	0.00	&	0.00	\\
79	&	0.04	&	0.00	&	0.00	&	0.00	&	0.00	&	0.00	&	0.00	&	0.00	&	0.00	\\
80	&	0.55	&	0.76	&	0.16	&	0.68	&	0.69	&	0.00	&	0.68	&	0.00	&	0.00	\\
81	&	0.55	&	0.76	&	0.12	&	0.68	&	0.69	&	0.00	&	0.68	&	0.00	&	0.00	\\
82	&	0.55	&	0.76	&	0.98	&	0.74	&	0.99	&	1.00	&	0.86	&	0.97	&	0.93	\\
83	&	0.55	&	0.76	&	1.00	&	0.68	&	0.97	&	1.00	&	0.82	&	1.00	&	1.00	\\
84	&	0.55	&	0.76	&	0.95	&	0.70	&	0.95	&	0.99	&	0.77	&	0.84	&	0.00	\\
85	&	0.55	&	0.76	&	0.99	&	0.66	&	0.89	&	1.00	&	0.74	&	0.92	&	0.56	\\
86	&	0.01	&	0.00	&	0.00	&	0.00	&	0.00	&	0.00	&	0.00	&	0.00	&	0.00	\\
87	&	0.55	&	0.76	&	0.88	&	0.70	&	0.71	&	0.94	&	0.67	&	0.64	&	0.00	\\
88	&	0.55	&	0.76	&	0.95	&	0.74	&	0.99	&	0.99	&	0.90	&	0.97	&	0.42	\\
89	&	0.55	&	0.76	&	0.17	&	0.68	&	0.42	&	0.00	&	0.46	&	0.00	&	0.00	\\
90	&	0.55	&	0.50	&	0.94	&	0.68	&	0.90	&	1.00	&	0.55	&	0.69	&	0.15	\\
91	&	0.55	&	0.76	&	0.78	&	0.74	&	0.96	&	0.03	&	0.53	&	0.01	&	0.00	\\
92	&	0.55	&	0.76	&	1.00	&	0.68	&	0.97	&	1.00	&	0.76	&	0.99	&	0.99	\\
93	&	0.55	&	0.76	&	0.76	&	0.72	&	0.90	&	0.00	&	0.69	&	0.02	&	0.00	\\
94	&	0.55	&	0.76	&	0.99	&	0.72	&	0.50	&	0.63	&	0.23	&	0.13	&	0.03	\\
95	&	0.55	&	0.76	&	1.00	&	0.64	&	0.94	&	1.00	&	0.78	&	0.99	&	1.00	\\
96	&	0.55	&	0.76	&	0.95	&	0.74	&	0.71	&	0.02	&	0.21	&	0.00	&	0.00	\\
97	&	0.55	&	0.76	&	0.99	&	0.66	&	0.83	&	0.81	&	0.56	&	0.54	&	0.03	\\
98	&	0.55	&	0.28	&	0.03	&	0.25	&	0.01	&	0.00	&	0.07	&	0.00	&	0.00	\\
99	&	0.55	&	0.76	&	0.93	&	0.72	&	0.96	&	1.00	&	0.89	&	0.99	&	0.23	\\
100	&	0.55	&	0.76	&	0.16	&	0.68	&	0.69	&	0.00	&	0.76	&	0.00	&	0.00	\\
101	&	0.55	&	0.76	&	0.26	&	0.70	&	0.89	&	0.00	&	0.70	&	0.00	&	0.00	\\
102	&	0.55	&	0.76	&	0.16	&	0.68	&	0.69	&	0.00	&	0.68	&	0.00	&	0.00	\\
103	&	0.55	&	0.76	&	0.89	&	0.74	&	0.75	&	0.01	&	0.31	&	0.00	&	0.00	\\
104	&	0.55	&	0.76	&	0.12	&	0.68	&	0.69	&	0.00	&	0.76	&	0.00	&	0.00	\\
105	&	0.55	&	0.53	&	0.44	&	0.53	&	0.82	&	0.00	&	0.78	&	0.02	&	0.00	\\
106	&	0.55	&	0.76	&	1.00	&	0.72	&	0.98	&	1.00	&	0.85	&	1.00	&	1.00	\\
107	&	0.55	&	0.50	&	0.01	&	0.38	&	0.02	&	0.00	&	0.20	&	0.00	&	0.00	\\
108	&	0.55	&	0.76	&	0.49	&	0.70	&	0.89	&	0.08	&	0.70	&	0.02	&	0.00	\\
109	&	0.55	&	0.76	&	0.12	&	0.68	&	0.69	&	0.00	&	0.68	&	0.00	&	0.00	\\

\end{longtable}
\end{center}
